# Supplementary material for: An Axiomatic Theory of Provably-Fair Welfare-Centric Machine Learning
Source: arXiv:2104.14504 source file (2021-07-26)
Supplement: Supplementary file 1 [file appendix_old.tex]

Here we present all missing proofs of results in the main text.

\subsection{Welfare and Malfare}
\label{sec:appx:proof:wm}


We now show \cref{thm:pow-mean-prop}.

\thmpowmeanprop*
%
\begin{proof}

\todo{Allow finitely-many region-breaks in the loss function (separate covers)}

We omit proof of \cref{thm:pow-mean-prop:mono}, as this is a standard property of power-means (generally termed the \emph{power mean inequality} \citep[chapter~3]{bullen2013handbook}).


%Lipschitz-Continuity: H\"older's inequality? Discrete formulation:

We first show \cref{thm:pow-mean-prop:subadditivity}.
By the triangle inequality (for $p \geq 1$), we have
\[
\Mean_{p}(\lv + \epsv; \wv) \leq \Mean_{p}(\lv; \wv) + \Mean_{p}(\epsv; \wv) \enspace.
\]
\if 0 %OLD
\[
\Mean_{p}(\lv + \epsv; \wv) = \sqrt[p]{\sum_{i=1}^{\NGroups} \wv_{i}(\lv_{i} + \epsv_{i})^{p}} = \norm{ \wv \otimes (\lv + \epsv) }_{p} \leq 
%\begin{array}{c} \norm{\wv}_{p}\norm{\lv + \epsv}_{p}????? \\ 
\norm{\wv \otimes \lv}_{p} + \norm{\wv \otimes \epsv}_{p} = \Mean_{p}(\lv; \wv) + \Mean_{p}(\epsv; \wv) %\end{array}
\]
\fi

We now show \cref{thm:pow-mean-prop:contraction}
First take $\epsv \doteq \lv - \lv'$.
Now consider
\begin{align*}
\Mean_{p}(\lv; \w) &= \Mean_{p}(\lv' + \epsv; \w) & \textsc{Definition of $\epsv$} \\
 &\leq \Mean_{p}(\lv' + \epsv_{+}; \w) & \textsc{Monotonicity} \\
 &\leq \Mean_{p}(\lv'; \wv) + \Mean_{p}(\epsv_{+}; \wv) & \textsc{\cref{thm:pow-mean-prop:subadditivity}} \\
 &\leq \Mean_{p}(\lv'; \wv) + \Mean_{p}(\abs{\lv - \lv'}; \wv) \enspace. & \textsc{Monotonicity} \\
\end{align*}
By symmetry, we have $\Mean_{p}(\lv', \wv) \leq \Mean_{p}(\lv, \wv) + \Mean_{p}(\abs{\lv - \lv'}; \wv)$, which implies the result.

\if 0
\todo{
For $p \leq -1$; we have
\[
\sqrt[p]{\Expect_{\omega \distributed \wv}[\lv^{p}(\omega)]} 
\]
}
\fi

We now show \cref{thm:pow-mean-prop:curvature}.
First note the special cases of $p \in \pm \infty$ follow by convexity of the maximum ($p=\infty$) and concavity of the minimum ($p=-\infty$).

Now, note that for $p \geq 1$, by concavity of $\sqrt[p]{\cdot}$, Jensen's inequality gives us 
\[
\Mean_{1}(\lv; \wv) = \Expect_{\omega \distributed \wv}[\lv(\omega)] = \underbrace{\Expect_{\omega \distributed \wv}[\sqrt[p]{\lv^{p}(\omega)}] \leq \sqrt[p]{\Expect_{\omega \distributed \wv}[\lv^{p}(\omega)]}}_{\textsc{Definition of Convexity}} = \Mean_{p}(\lv; \wv) \enspace,
\]
i.e., convexity, and similarly, for $p \leq 1$, $p \neq 0$, we have by convexity of $\sqrt[p]{\cdot}$, we have
\[
\Mean_{1}(\lv; \wv) = \Expect_{\omega \distributed \wv}[\lv(\omega)] = \underbrace{\Expect_{\omega \distributed \wv}[\sqrt[p]{\lv^{p}(\omega)}] \geq \sqrt[p]{\Expect_{\omega \distributed \wv}[\lv^{p}(\omega)]}}_{\textsc{Definition of Concavity}} = \Mean_{p}(\lv; \wv) \enspace.
\]
Similar reasoning, now by convexity of $\ln(\cdot)$, shows the case of $p=0$. %, which completes the proof.%\todo{show more detail?}
%
\end{proof}


We now show \cref{thm:pop-mean-prop}.

\thmpopmeanprop*
%
\begin{proof}

%1
\Cref{thm:pop-mean-prop:id} is an immediate consequence of axioms
\ref{def:cardinal-axioms:mult} \& \ref{def:cardinal-axioms:unit} (multiplicative linearity and unit scale).
%\todo{proof detail?}

%Old 2
%To see $\Mean(\lv) \leq \Mean_{\infty}(\lv)$, note that $\Mean(\bm{0}) = 0$ (by item 1), thus by axiom 8, $\Mean(\lv) \leq \norm{\lv}_{\infty} = \max \lv = \Mean_{\infty}(\lv)$.
%\todo{use min instead of 0 to extend to nonnegs}

%2
We now note that \cref{thm:pop-mean-prop:lin-fact} is the celebrated Debreu-Gorman theorem \citep{debreu1959topological,gorman1968structure}, extended by continuity and measurability of $\lv$ to the weighted case.\todo{see also for more on Debreu-Gorman: Wakker, P.P., 1989. Additive Representations of Preferences; may need less than continuity?}



%3
We now show \cref{thm:pop-mean-prop:pmean}.\todo{Properly show the split; w/ and w/out scale.}
This result is essentially a corollary of \cref{thm:pop-mean-prop:lin-fact}, hence the dependence on axioms 1-4.
\todo{
We now assume axiom \ref{def:cardinal-axioms:mult}, and the task is to prove $F(u) = \alpha\sqrt[p]{\sgn(p)u}$. %%$F(u) = \alpha\sqrt[p]{\sgn(p)u + \beta^{p}} - \beta$?
}%
%
%
Suppose $\lv(\cdot) = 1$.  %, and take $\Mean(\lv; \wv) = c$.
By \cref{def:cardinal-axioms:mult} and \cref{def:cardinal-axioms:unit}, 
for all $p \neq 0$, we have:
\[
\alpha = \alpha\Mean(\lv; \wv)
  = \Mean(\alpha\lv; \wv)
  = F(\Expect_{\omega \distributed \wv}[f_{p}(\alpha\lv(\omega))])
  = F(\Expect_{\omega \distributed \wv}[f_{p}(\alpha)])
  = \begin{cases} p > 0 & \displaystyle F(\Expect_{\omega \distributed \wv}[(\alpha\lv(\omega))^{p}]) = F(\alpha^{p}) \\ p < 0 & \displaystyle F(\Expect_{\omega \distributed \wv}[-(\alpha\lv(\omega))^{p}]) = F(-\alpha^{p}) \\ \end{cases} \enspace.
\]
From here, it is clear that for $p > 0$, $\alpha = F(\alpha^{p})$, thus $F^{-1}(u) = u^{p}$ and consequently $F(v) = \sqrt[p]{v}$, and similarly, for $p < 0$, $\alpha = F(-\alpha^{p})$, thus $F^{-1}(u) = -u^{p}$, and consequently $F(v) = \sqrt[p]{-v}$.


%Older; long-winded proof
\if 0
\[
1 = \Mean(\lv; \wv) = F(\Expect_{\omega \distributed \wv}[f_{p}(\lv(\omega))] = F(1)
\]

\[
\alpha = \alpha\Mean(\lv; \wv) = \Mean(\alpha\lv; \wv) = F(\Expect_{\omega \distributed \wv}[f_{p}(\alpha\lv(\omega))]) = F(\alpha^{p})
\]

\todo{Isn't it obvious from 2nd form?}

Now, we apply $F^{-1}$ to both sides of both equations and divide \todo{check / 0}:

\[
\frac{F^{-1}(\alpha)}{F^{-1}(1)} = \alpha^{p}
\]

Now, note that $F(1) = 1$, thus $F^{-1}(1) = 1$, which leaves
\[
F^{-1}(\alpha) = \alpha^{p} \implies F(\alpha) = \sqrt[p]{\alpha} \enspace.
\]

\todo{Show what happens without assuming unit scale (commented) and other cases of $p$.  It's just $F(\alpha) = \sqrt[p]{\alpha / F^{-1}(c)}$; $F^{-1}(c)$ is just some nonneg constant.}
\fi



Taking $p = 0$ gets us
\if 0
\[
1 = \Mean(\lv; \wv) = F(\Expect_{\omega \distributed \wv}[\ln(\lv(\omega))]) = F(0)
\]
\fi

\[
\alpha = \alpha\Mean(\lv; \wv) = F(\Expect_{\omega \distributed \wv}[\ln(\alpha\lv(\omega))]) = F(\ln a) \enspace,
\]
from which it is clear that $F^{-1}(u) = \ln(u) \implies F(v) = \exp(v)$.

In all cases of $p$, substituting the values of $f_{p}$ and %$F_{p}$
$F(\cdot)$ %TODO F_{p}
into \ref{thm:pop-mean-prop:lin-fact} yields $\Mean(\lv; \wv) = \Mean_{p}(\lv; \wv)$.

\if 0
Finally, for the case of $p < 0$, taking $G(u) = F(-u)$, we get
\[
\alpha = \alpha\Mean(\lv; \wv) = \Mean(\alpha\lv; \wv) = F(\Expect_{\omega \distributed \wv}[f_{p}(\alpha\lv(\omega))] = G(-\alpha^{p}) = F(\alpha^{p}) \enspace,
\]
and the rest proceeds as in the case of $p > 0$.
\fi

%Very old, very wrong proof
%Axiom 5 then implies $\Mean(\lv) \propto \Mean_{p}(\lv)$\todo{prove it?}.
%Finally, axiom \cref{def:cardinal-axioms:unit} implies $\alpha = 1$.

%4&5
We now show \ref{thm:pop-mean-prop:pmean-fair} and \ref{thm:pop-mean-prop:pmean-unfair}.
These properties follow directly from \ref{thm:pop-mean-prop:lin-fact}, wherein $f_{p}$ are defined, and Jensen's inequality. %, wherein we see that  %TODO give more detail?
\todo{prove this in detail.}
%PD transfer implies $\Mean_{1}(\lv) \leq \Mean(\lv)$, because $\Mean_{1}(\lv) = \Mean_{1}(\mu) \leq_{PD} \Mean(\lv)$.


\end{proof}



We now show \cref{coro:stat-est}.
\corostatest*
\begin{proof}
This result is a corollary of \cref{lemma:stat-est}, applied to $\epsv$, where we note that for $p \geq 1$, by \cref{thm:pow-mean-prop}~item~\ref{thm:pow-mean-prop:contraction} (contraction)
it holds that
\[
\Mean_{p}(\hat{\lv} + \epsv; \wv) \leq \Mean_{p}(\hat{\lv}; \wv) + \norm{\epsv}_{\infty} \ \& \ \Mean_{p}(\bm{0} \vee (\hat{\lv} - \epsv); \wv) \leq \Mean_{p}(\hat{\lv}; \wv) - \norm{\epsv}_{\infty} \enspace.
\]

Now, for the first bound, note that we take $\epsv_ {i} \doteq \frange\sqrt{\frac{\ln \frac{2\NGroups}{\delta}}{2m}}$, and by Hoeffding's inequality and the union bound, for $\Omega = \{1, \dots, n\}$, we have $\forall \omega: \, \lv'(\omega) - \epsv(\omega) \leq \lv(\omega) \leq \lv'(\omega) + \epsv(\omega)$ with probability at least $1 - \delta$.
The result then follows via the \emph{power-mean contraction} (\cref{thm:pow-mean-prop} item \ref{thm:pow-mean-prop:contraction}) property.

Similarly, for the second bound, note that we take $\epsv_ {i} \doteq \frac{\frange\ln \frac{2\NGroups}{\delta}}{3m} + %\sup_{i \in 1, \dots, \NGroups}
\sqrt{\frac{2\Var_{\ProbDist_{i}}[\LossFunction] \ln \frac{2\NGroups}{\delta}}{m}}$, which this time follows via Bennett's inequality and the union bound.
Now, we again apply \cref{lemma:stat-est}, noting that $\Mean(\epsv) \leq \Mean_{\infty}(\epsv) = \norm{\epsv}_{\infty}$ (by \emph{power-mean monotonicity}, \cref{thm:pow-mean-prop:mono} item \ref{thm:pow-mean-prop:mono}), and the rest follows as in the Hoeffding case.
% and the rest is as with the Hoeffding case. % (note that here thus the \rhs{} is $\norm{\epsv}_{\infty}$).
%\todo{improvement: 1 side is direct by concavity convextity: $2n$ could be $n+1$?}
\end{proof}
%The above bound is a straightforward consequence of Hoeffding's inequality; similar variance-sensitive bounds can be shown with Bennett's inequality, and uniform convergence bounds with Rademacher averages.



\subsection{Efficient FPAC-Learning}
\label{sec:appx:proof:efpac}


We now show \cref{thm:aemm-psg}.

\thmaemmpsg*
\begin{proof}
%
We now show that this subgradient-method construction of $\PACAlgo$ requires $\Poly(\frac{1}{\varepsilon}, \frac{1}{\delta}, \DSeq, \NGroups)$ time to identify an $\varepsilon$-$\delta$-$\Malfare_{p}(\dots)$-optimal $\theta \in \Theta_{\DSeq}$, and thus fair-PAC-learns $(\HC, \LossFunction)$.
This essentially boils down to showing that the empirical malfare objective \todo{state here} is \emph{convex}\todo{show me}, \emph{Lipschitz}, and \emph{bounded}, and that \cref{alg:aemm-psg} runs sufficiently many steps with appropriate step size, on a sufficiently large training set, to yield the appropriate guarantees, and that each step of the subgradient method, of which there are polynomially many, itself requires polynomial time.

As above, take $\SampleComplexity_{\PACAlgo} \doteq \SampleComplexity_{\mathrm{UC}}({\frac{\varepsilon}{2}}, \frac{\delta}{\NGroups}, \DSeq)$.
\todo{Explain why $m$, fix form}

First note that evaluating a subgradient (via forward finite-difference estimation\cyrus{This may be a (fixable) source of error not accounted for?}) requires $(\dim(\Theta_{\DSeq}) + 1) \SampleComplexity_{\PACAlgo}$ evaluations of $h(\cdot; \cdot)$, which by assumption is possible in $\Poly(\DSeq, \SampleComplexity_{\PACAlgo}) = \Poly(\frac{1}{\varepsilon}, \frac{1}{\delta}, \DSeq, \NGroups)$ time.

Now, note that for any $p$, $\wv$,
\[
\forall \lv, \lv': \ \abs{\Malfare_{p}(\lv; \wv) - \Malfare_{p}(\lv'; \wv)}  \leq 1 \norm{\lv - \lv'}_{\infty} \enspace,
\]
i.e., $\Malfare_{p}(\cdot; \wv)$ is $1$-$\norm{\cdot}_{\infty}$-$\abs{\cdot}$-Lipschitz (see \cref{thm:pow-mean-prop}, item~\ref{thm:pow-mean-prop:contraction}), and thus by Lipschitz composition, we thus have Lipschitz property %obeys the Lipschitz condition
\[
\forall \theta, \theta' \in \Theta_{\DSeq}: \ \abs{ \Malfare \bigl( i \mapsto \ERisk(h(\cdot; \theta); \wv \bigr) - \Malfare \bigl( i \mapsto \ERisk(h(\cdot; \theta'); \wv \bigr) } \leq \lambda_{\LossFunction}\lambda_{\HC}\norm{\theta - \theta'}_{2} \enspace. \todo{fixme}
\]
\todo{subscript or ; on theta?}

\todo{sth like:
\[
\Malfare \bigl( i \mapsto \ERisk(h(\cdot; \theta); \LossFunction, \bm{x}_{i}); \wv \bigr) \leq \Malfare \bigl( i \mapsto \Risk(h(\cdot; \theta); \LossFunction, \ProbDist_{i}); \wv \bigr) + \varepsilon
\]
}

The subgradient method produces $\hat{\theta}$ such that \citep[see][]{shor2012minimization}
\[
f(\theta) \leq f(\theta^{*}) + \frac{\norm{\theta_{0}, \theta^{*}}^{2}_{2} + \Lambda^{2}\alpha^{2}n}{2 \alpha n} \leq \frac{\Diam^{2}(\Theta_{\DSeq}) + \Lambda^{2}\alpha^{2}n}{2 \alpha n} \enspace,
\]
for $\Lambda$-$\norm{\cdot}_{2}$-$\abs{\cdot}$-Lipschitz objective $f$, thus taking %$\alpha \doteq \frac{\norm{\theta_{0}, \theta^{*}}_{2}}{\Lambda\sqrt{n}}$
$\alpha \doteq \frac{\Diam(\Theta_{\DSeq})}{\Lambda\sqrt{n}}$ 
yields
\[
f(\theta) - f(\theta^{*}) \leq \frac{\Diam(\Theta_{\DSeq})\Lambda}{\sqrt{n}} \enspace.
\]

\if 0
thus taking $\alpha = n^{-1/2}$ yields
\[
\leq f(\theta^{*}) + \frac{\norm{\theta_{0}, \theta^{*}}^{2}_{2} + \Lambda^{2}}{2\sqrt{n}} \enspace.
\]
\fi


As shown above, $\Lambda = 1 \lambda_{\LossFunction} \lambda_{\HC}$, thus we may guarantee \emph{optimization error}
\[
\varepsilon_{opt} \doteq f(\hat{\theta}) - f(\theta^{*}) \leq \frac{\varepsilon}{2}
\]
if we take iteration count
\if 0 %Using bad alpha:
\[
n \geq \frac{\Diam(\Theta_{\DSeq})^{4} + \lambda_{\LossFunction}^{4}\lambda_{\HC}^{4}}{\varepsilon^{2}} \in \Poly(\mathsmaller{\frac{1}{\varepsilon}}, \DSeq) \enspace.
\]
\fi
\[
n \geq \frac{4\Diam^{2}(\Theta_{\DSeq})\lambda_{\LossFunction}^{2}\lambda_{\HC}^{2}}{\varepsilon^{2}} = \left(\frac{2\Diam(\Theta_{\DSeq})\lambda_{\LossFunction}\lambda_{\HC}}{\varepsilon}\right)^{2} \in \Poly(\mathsmaller{\frac{1}{\varepsilon}}, \DSeq) \enspace.
\]



As each iteration requires $\SampleComplexity_{\PACAlgo}\Poly(\DSeq) \subseteq \Poly(\frac{1}{\varepsilon}, \frac{1}{\delta}, \DSeq, \NGroups)$ time, %the total time complexity of running the subgradient method for $n$ iterations is 
%It thus holds that, via
the subgradient method identifies a ${\frac{\varepsilon}{2}}$-empirical-malfare-optimal $\hat{\theta} \in \Theta_{\DSeq}$ in
\if 0
\[
n \in \Poly(\frac{1}{\varepsilon}) \Poly(\DSeq) \subseteq \Poly(\frac{1}{\varepsilon}, \frac{1}{\delta}, \DSeq, \NGroups)
\]
subgradient-method steps, each requiring $\SampleComplexity_{\PACAlgo}\Poly(\DSeq) \subseteq \Poly(\frac{1}{\varepsilon}, \frac{1}{\delta}, \DSeq, \NGroups)$ time, thus totaling 
\fi
$\Poly(\frac{1}{\varepsilon}, \frac{1}{\delta}, \DSeq, \NGroups)$ time.

As $\SampleComplexity_{\PACAlgo}$ was selected to ensure $\frac{\epsilon}{2}$-$\frac{\delta}{\NGroups}$ uniform convergence, we thus have that by uniform convergence, and union bound (over $\NGroups$ groups), with probability at least $1 - \delta$, the EMM-optimal $\tilde{h}$ obeys
\cyrus{The next few bounds are slightly off; easily fixable.}
\[
\Malfare(i \mapsto \ERisk(\tilde{h}; \loss, \bm{x}_i); \wv) \leq \Malfare(i \mapsto \Risk(h; \loss, \ProbDist_i); \wv) + \frac{\varepsilon}{2}
\todo{\dots} \leq \epsilon \enspace.
\]
Similarly, we have
\[
\Malfare(i \mapsto \ERisk(\hat{h}; \loss, \bm{x}_i); \wv) \leq \Malfare(i \mapsto \ERisk(\tilde{h}; \loss, \bm{x}_i); \wv) + \frac{\varepsilon}{2}
\]
Combining \emph{estimation} and \emph{optimization} errors, we get that with probability at least $1 - \delta$, \todo{and applying LIPSCHITZ MALFARE}
\[
\Malfare(i \mapsto \ERisk(\hat{h}; \loss, \bm{x}_i); \wv) \leq \Malfare(i \mapsto \ERisk(\tilde{h}; \loss, \bm{x}_i); \wv) + \frac{\varepsilon}{2} \leq \Malfare(i \mapsto \Risk(h; \loss, \ProbDist_i); \wv) + \varepsilon \enspace.
\]
\cyrus{Detail: I think we need to account for bidirectional UC error, so need to change fractions to 1/3 each error source?}

We may thus conclude that $\PACAlgo$ fair-PAC learns $\HC$, and consequently, $(\HC, \ell) \in \PAC^{\Agnostic}_{\Poly}$.
\end{proof}







We now show \cref{thm:aemm-covering}.
\thmaeemcovering*
\begin{proof}
We now constructively show the existence of a fair-PAC-learning algorithm $\PACAlgo$ for $\HC$ and $\loss$ over domain $\X$ and codomain $\Y$.
\if 0
First take \emph{cover precision} $\gamma \doteq \frac{\varepsilon}{3D_{\Y}\lambda_{\loss}}$\todo{/range}.

\cyrus{Should be more like $\gamma \doteq \frac{\varepsilon}{3(\LossFunction_{\infty} + \lambda_{\loss})}$}

\cyrus{Actually just need $\gamma \doteq \frac{\varepsilon}{3\lambda_{\loss}}$}
\fi 
First take \emph{cover precision} $\gamma \doteq \frac{\varepsilon}{6\lambda_{\loss}}$.
We now construct a training sample $\bm{x}_{1:\NGroups,1:m}$ consisting of $m$ draws from each of the $\NGroups$ groups (we shall later show that $m \in \Poly(\frac{1}{\varepsilon}, \frac{1}{\delta}, \DSeq, \NGroups)$ is sufficient).
By assumption, we may enumerate a cover $\Cover(\HC_{\DSeq}, \bm{x}, \gamma)$ in $\Poly(m, \nicefrac{1}{\gamma}, \DSeq) = \Poly(m, \frac{4\lambda_{\loss}}{\varepsilon}, \DSeq) = \Poly(m, \frac{1}{\varepsilon}, \DSeq)$ time. % (we shall later show that $m \in \Poly(\frac{1}{\varepsilon}, \frac{1}{\delta}, \DSeq, \NGroups)$ to complete the desideratum).
%, which is $\Poly(m, \nicefrac{1}{\varepsilon})$, as $3D_{\Y}\lambda_{\loss}$ is constant.
%\todo{suffices to cover w.h.p.?}
\todo{Detail: need to cover $\cup_{i=1}^{\NGroups} \bm{x}_{i}$, with $\gamma$ precision each, which means sth like $\gamma/\NGroups$ precision?  Alternatively, take a \emph{union} over per-group covers?} 
The learning algorithm is thus \emph{empirical malfare minimization} over $\hat{\Cover}(\HC_{\DSeq}, \bm{x}, \gamma)$.
Let
\[
\hat{h} \doteq \argmin_{h \in \hat{\Cover}(\HC_{\DSeq}, \bm{x}, \gamma)} \Malfare_{p}(i \mapsto \ERisk(h; \bm{x}_i); \wv) %$. \& 
\ \ \ \& \ \ \ \tilde{h} \doteq \argmin_{h \in \HC} \Malfare_{p}(i \mapsto \ERisk(h; \bm{x}_i); \wv) \enspace,%$. \&
\]
where ties may be broken arbitrarily.
%\todo{argmin or something that denotes breaking ties?}
\todo{x vs xi; union?}
By Lipschitz and covering properties, we thus bound the \emph{optimization error} as
\[
\varepsilon_{opt}
  \doteq \Malfare_{p}(i \mapsto \ERisk(\hat{h}; \bm{x}_i); \wv) - \Malfare(i \mapsto \ERisk(\tilde{h}; \bm{x}_i); \wv)
  \leq \gamma \lambda_{\loss}
  \enspace.
\]
%
This controls for \emph{optimization error} between the true and approximate EMM solutions $\tilde{h}$ and %approximate EMM solution 
$\hat{h}$.

\todo{Because $\Cover(\HC_{\DSeq}, \bm{x}, \gamma)$ not fixed a priori...}

We now quantify the \emph{approximation error} (due to sampling) for any $h \in \HC$ as
\if 0
\[
\argmin_{\tilde{h} \in \HC }  \Malfare()  \leq \argmin_{h^{*}} \Malfare() ? 
\]
\fi
\begin{align*}
\epsilon_{apx}
  &= \Malfare(i \mapsto \ERisk(h; \loss, \bm{x}_i); \wv) - \Malfare(i \mapsto \Risk(h; \loss, \ProbDist_i); \wv) & \\
  &\leq \max_{i \in 1, \dots, \NGroups} \abs{ \Risk(\hat{h}; \loss, \ProbDist_i); \wv) - \ERisk(\hat{h}; \loss, \bm{x}_i); \wv) } \\
  &\leq %\lambda_{\loss} \left(
  \underbrace{2\lambda_{\loss} \gamma}_{\textsc{Discretization}} + 2\underbrace{\loss_{\infty}\sqrt{\frac{\ln \Covering(\HC_{\DSeq}, m, \gamma) }{2m}}}_{\textsc{Entropy}} + \underbrace{%\norm{\loss}_{\infty}
  %D_{\Y}\lambda_{\loss}
  \loss_{\infty}\sqrt{\frac{\ln \frac{\NGroups}{\delta}}{2m}}}_{\textsc{SD / $\Malfare(\cdot; \cdot)$ Tail Bound}} %\right) \leq ?
  %\leq \varepsilon
  \enspace, & \\
\end{align*}
which follows as a direct consequence of discretization and Massart's finite class lemma to bound the (per-group) expected suprema of deviations, followed by McDiarmid's inequality and a union bound to bound the suprema of deviations \wrt{} the sample $\bm{x}_{1:m}$, and \cref{lemma:stat-est} and \cref{thm:pow-mean-prop:contraction} (item \ref{thm:pow-mean-prop:contraction}) to translate these risk bounds into malfare bounds.\cyrus{Lots of detail missing there.}
Note that we base the bounds on the \emph{covering number} $\Covering(\HC_{\DSeq}, m, \gamma)$, which bound the size of the optimal (perhaps unknown) empirical cover $\Cover^{*}(\HC_{\DSeq}, \bm{x}, \gamma)$; similar bounds are possible using $\abs{\hat{\Cover}(\HC_{\DSeq}, \bm{x}, \gamma)}$, at a constant-factor cost to sample complexity. 
%The same holds for $h^{*}$, ...
%\cyrus{Key step: $D_{\loss} \leq D_{\Y}\lambda_{\loss}$?}

Combining the optimization and sampling error inequalities, take $\epsilon_{m} \doteq \Malfare(i \mapsto \Risk(h^{*}; \loss, \ProbDist_i); \wv) - \Malfare(i \mapsto \Risk(\hat{h}; \loss, \ProbDist_i); \wv)$, and note
\begin{align*}
  \epsilon_{m}
  &= \left(\Malfare(i \mapsto \Risk(h^{*}; \loss, \ProbDist_i); \wv) -  \Malfare(i \mapsto \ERisk(h^{*}; \loss, \bm{x}_i); \wv)\right) & \leq \epsilon_{apx} \\
    %& \ \ + \left(\Malfare(i \mapsto \ERisk(h^{*}; \loss, \bm{x}_i); \wv) -  \Malfare(i \mapsto \ERisk(h^{*}; \loss, \bm{x}_i); \wv)\right) & \leq ? \\
    & \ \ + \left(\Malfare(i \mapsto \ERisk(h^{*}; \loss, \bm{x}_i); \wv) -  \Malfare(i \mapsto \ERisk(\tilde{h}; \loss, \bm{x}_i); \wv)\right) & \leq 0 \\
    & \ \ + \left(\Malfare(i \mapsto \ERisk(\tilde{h}; \loss, \bm{x}_i); \wv) - \Malfare(i \mapsto \ERisk(\hat{h}; \loss, \bm{x}_i); \wv) \right) & \leq \epsilon_{opt} \\
    & \ \ + \left(\Malfare(i \mapsto \ERisk(\hat{h}; \loss, \bm{x}_i); \wv) - \Malfare(i \mapsto \Risk(\hat{h}; \loss, \ProbDist_i); \wv)\right) & \leq \epsilon_{apx} \\
  &\leq \epsilon_{opt} + 2\epsilon_{apx} & \\
  &= 5\gamma \lambda_{\loss} + 4\loss_{\infty}\sqrt{\frac{\ln \Covering(\HC_{\DSeq}, m, \gamma) }{2m}} + 4\loss_{\infty}\sqrt{\frac{\ln \frac{\NGroups}{\delta}}{2m}} & \\
  &\leq \frac{5}{6} \varepsilon + 8\loss_{\infty} \sqrt{\frac{\ln \Covering(\HC_{\DSeq}, m, \gamma)\ln \frac{\NGroups}{\delta}}{2m}} \enspace. & \forall a, b \geq 1: \ \sqrt{a} + \sqrt{b} \leq 2\sqrt{ab} \\
\end{align*}

\todo{Last step assumes $\delta$ is small.}

Now, select the smallest $m \in \N$ such that the \rhs{} is no greater than $\varepsilon$, and note that $m \in \Poly( \frac{1}{\varepsilon}, \ln \frac{\NGroups}{\delta}, \ln \Covering(\HC_{\DSeq}, m, \gamma) ) \subset \Poly(\frac{1}{\varepsilon}, \frac{1}{\delta}, \NGroups, \DSeq)$, essentially because, by assumption, $\ln \Covering(\HC_{\DSeq}, m, \gamma) \in \ln \Poly(m, \frac{1}{\gamma}, \DSeq)$\todo{Better notation for $\log \circ \Poly$?  Just $\LandauO \log(\dots)$?}. % \subseteq  \Poly(\dots)$, 
%and the McDiarmid tail bound terms.
%Now pick $m$ as smallest $m$ s.t. $\sqrt{\dots} = \eps/3$, wh.??? $m \in \Poly(?)$.


We thus conclude that both the sample complexity and time complexity of this algorithm are $\Poly(\frac{1}{\varepsilon}, \ln \frac{\NGroups}{\delta}, \NGroups, \DSeq)$.
Hence, as we have constructed a polynomial-time fair-PAC learner for $(\HC, \LossFunction)$, we may conclude $(\HC, \LossFunction) \in \FPAC_{\Poly}$.
%
%Dudley discretization argument (essentially Massart's lemma).
\todo{Are conditions applied by UC always via Sudakov?}
%
\todo{assume computability to evaluate}
%
\todo{Agnostic / realizable cases?}
\fi
%
\end{proof}
